# Supplementary material for: HadamRNN: Binary and Sparse Ternary Orthogonal RNNs
Source: arXiv:2502.00047 source file (2025-05-06)
Supplement: Supplementary file 1 [file binary_connect.tex]

\section{Details on \textit{BinaryConnect} \cite{10.5555/2969442.2969588}}
\label{app:binary_connect}

The BinaryConnect algorithm is used to train neural networks with $\{-1,1\}$ weights. Let $W$ be a $n \times m$ weight matrix with $\pm 1$ values. The main idea is to associate a real-valued \textit{latent weight} matrix $\Tilde{W} \in \RR^{n \times m}$ to $W$. Forward propagation is calculated using $W$, and gradient updates are made at $\Tilde{W}$ using the gradient of the loss computed at the binary point $W$.

More specifically, assume $t$ training iterations of our network have yielded a latent weight matrix $\Tilde{W}_t$. $W_t$ is binarized as $W_t = sgn(\Tilde{W}_t)$, where $sgn(.)$ denotes the sign function applied coordinate-wise. The loss $L$ is calculated at iteration $t+1$ using $W_{t}$ and the other current parameters. During backpropagation, we compute the gradient of the loss $g$ with respect to \textbf{the binary weight} $W_t$:
$$
g = \frac{\partial L}{\partial W_t},
$$
and the update is made at \textbf{the latent weight} $\Tilde{W}_t$:
$$
\Tilde{W}_{t+1} = \Tilde{W}_t - \eta_t g,
$$
where $\eta_t$ is the current learning rate, and assuming optimization is made through a simple stochastic gradient descent step. However, this update scheme can be easily generalized to any other classic optimizer such as RMSprop or Adam.
