# Supplementary material for: HadamRNN: Binary and Sparse Ternary Orthogonal RNNs
Source: arXiv:2502.00047 source file (2025-05-06)
Supplement: Supplementary file 2 [file rnn_gradient.tex]

\section{On the assumption that $D_k$ has close to $1$ diagonal entries}
\label{appendix:rnn_grad}
