# Supplementary material for: HadamRNN: Binary and Sparse Ternary Orthogonal RNNs
Source: arXiv:2502.00047 source file (2025-05-06)
Supplement: Supplementary file 3 [file vRNN_binary_difficult.tex]

\section{On the difficulty of training vanilla RNNs}
\label{appendix:binary_vrnn_difficult}
